# Supplementary material for: Topological defects in spiral wave chimera states
Source: arXiv:2511.21058 ancillary file (2026-03-05)
Supplement: Supplementary file 1 [file Supplemental_Material.pdf]

# Supplemental Material for: “Topological Defects in Spiral Wave Chimera States”

Lintao Liu and Nariya Uchida\*

*Department of Physics, Tohoku University, Sendai 980-8578, Japan*

(Dated: November 26, 2025)

## OVERVIEW

This Supplemental Material provides additional details on the Linear Stability Analysis, the asymptotic behavior of the order parameter, the derivation of the Complex Ginzburg-Landau equation (CGLE), and the entropy hypothesis.

### S1. LINEAR STABILITY ANALYSIS

In this section, we briefly recapitulate the linear stability analysis of the  $q$ -twisted states (plane waves). It is straightforward to verify that the system admits traveling wave solutions of the form [1, 2]

$$\psi(\mathbf{r}, t) = \Omega t + \mathbf{Q} \cdot \mathbf{r}, \quad (\text{S1})$$

where  $\mathbf{Q}$  is the wave vector,  $\Omega$  is the corresponding frequency, and  $\mathbf{r} = (i, j)$  denotes the 2D lattice coordinates.

We introduce a small perturbation to this solution:

$$\psi(\mathbf{r}, t) = \Omega t + \mathbf{Q} \cdot \mathbf{r} + \sum_{\mathbf{K}} A_{\mathbf{K}} e^{i\mathbf{K} \cdot \mathbf{r} + \Lambda_{\mathbf{K}} t}, \quad (\text{S2})$$

where  $\mathbf{K} = \frac{2\pi}{N}(k_i, k_j)$  ( $k_i, k_j = 1, 2, \dots, N-1$ ), and  $A_{\mathbf{K}} \ll 1$  is the amplitude of the perturbation mode with the corresponding growth rate  $\Lambda_{\mathbf{K}}$ . The solution is linearly stable if the real part of the growth rate,  $\text{Re}(\Lambda_{\mathbf{K}})$ , is negative for all perturbation wave vectors  $\mathbf{K}$ .

Substituting the perturbed solution into the governing equation yields the zeroth-order equation:

$$\Omega = -\frac{1}{N} \sum_{\Delta \mathbf{r}} \sin(-\mathbf{Q} \cdot \Delta \mathbf{r} + \alpha), \quad (\text{S3})$$

and the first-order equation:

$$\begin{aligned} \sum_{\mathbf{K}} \Lambda_{\mathbf{K}} A_{\mathbf{K}} e^{i\mathbf{K} \cdot \mathbf{r} + \Lambda_{\mathbf{K}} t} &= -\frac{1}{N} \sum_{\Delta \mathbf{r}} \cos(-\mathbf{Q} \cdot \Delta \mathbf{r} + \alpha) \\ &\times \sum_{\mathbf{K}} A_{\mathbf{K}} e^{i\mathbf{K} \cdot \mathbf{r} + \Lambda_{\mathbf{K}} t} (1 - e^{i\mathbf{K} \cdot \Delta \mathbf{r}}), \end{aligned} \quad (\text{S4})$$

where  $\Delta \mathbf{r} = \mathbf{r}_{kl} - \mathbf{r}_{ij}$ . Simplifying this expression, we obtain the real part of the growth rate:

$$\text{Re}(\Lambda_{\mathbf{K}}) = -\frac{1}{N} \cos \alpha \sum_{\Delta \mathbf{r}} \cos(\mathbf{Q} \cdot \Delta \mathbf{r}) (1 - \cos(\mathbf{K} \cdot \Delta \mathbf{r})). \quad (\text{S5})$$

Applying the continuum approximation and appropriate rescaling [2], this discrete sum can be transformed into the following integral:

$$\text{Re}(\Lambda_{\mathbf{K}}) = -\frac{2 \cos \alpha}{\pi} \int_{|\Delta \mathbf{r}| \leq 1} \cos(\boldsymbol{\rho} \cdot \Delta \mathbf{r}) \sin^2 \left( \frac{\boldsymbol{\Xi} \cdot \Delta \mathbf{r}}{2} \right) d\Delta \mathbf{r}, \quad (\text{S6})$$

---

\* [nariya.uchida@tohoku.ac.jp](mailto:nariya.uchida@tohoku.ac.jp)

where  $\boldsymbol{\rho} = R\mathbf{Q}$ ,  $\boldsymbol{\Xi} = R\mathbf{K}$  are the rescaled wave vectors. Evaluating the integrals for the frequency (from Eq. S3) and the growth rate (from Eq. S6) yields the final forms:

$$\Omega = -2\pi \sin \alpha \frac{J_1(\rho)}{\rho}. \quad (\text{S7})$$

$$\begin{aligned} \text{Re } \Lambda(\rho, \Xi) &= -2 \cos \alpha \left[ \frac{J_1(\rho)}{\rho} - \frac{1}{2} \left( \frac{J_1(s_+)}{s_+} + \frac{J_1(s_-)}{s_-} \right) \right], \\ &= 2 \cos \alpha \left( \frac{J_1(\rho + \Xi)}{\rho + \Xi} - \frac{J_1(\rho)}{\rho} \right). \end{aligned} \quad (\text{S8})$$

where  $J_1$  is the Bessel function of the first kind of order one and  $s_{\pm} = |\boldsymbol{\rho} \pm \boldsymbol{\Xi}|$ , and we set  $\theta = \angle(\boldsymbol{\rho}, \boldsymbol{\Xi}) = 0$  for simplicity.

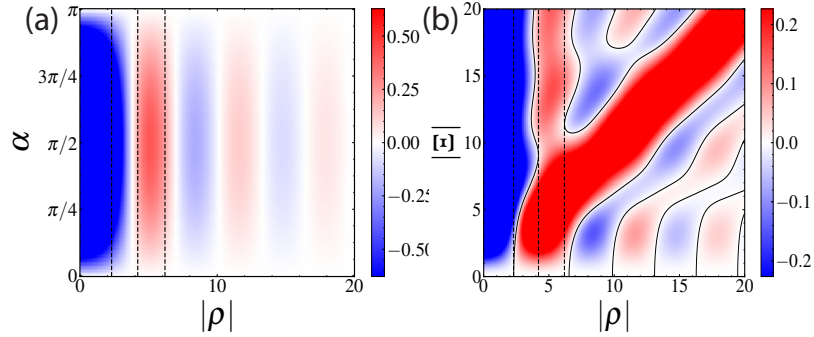

FIG. S1. (a) The phase velocity of the plane wave given by Eq. (S3). (b) The normalized linear growth rate  $\text{Re}(\Lambda_K)/\cos \alpha$  given by Eq. (S6). In both panels, the colormap spans  $\frac{1}{2}$  of the full range of the corresponding quantity.

Our result aligns well with the one-dimensional case reported in [1]. The stability of the twisted state is highly dependent on the phase lag  $\alpha$ , forming two distinct regimes. As shown in Fig. S1(b), when  $0 < \alpha < \frac{1}{2}\pi$  (the in-phase regime), the stable domain is determined to be in the approximate range of  $0 < \rho < 2.2917$ . when  $\frac{1}{2}\pi < \alpha < \pi$  (the anti-phase regime), the stable domain is determined to be in the approximate range of  $4.2005 < \rho < 6.1876$ . Given the relationship  $Q = \rho/R$  and assuming  $R = 6$ , these  $\rho$ -intervals translate to stable wavenumber ranges of approximately  $0 < Q < 0.122\pi$  and  $0.223\pi < Q < 0.328\pi$ , respectively.

The stable range narrows as  $R$  increases, which is interpreted as the result of frustration between many oscillators. Furthermore, for the  $\frac{1}{2}\pi < \alpha < \pi$  regime, we observe that the linearly stable range roughly corresponds to a band of positive phase velocity [cf. Fig. S1(a)]. This allows us to relate the stability to the frequency Eq. (S7). Thus, the existence of stable twisted states is a consequence of the finite interaction range.

## S2. ANALYSIS OF THE ORDER PARAMETER

The order parameter is defined as:

$$A_0(r) = \frac{1}{\pi R^2} \int_{(R-r)^2}^{(R+r)^2} \sqrt{1 - \frac{(r^2 + u - R^2)^2}{4r^2 u}} du. \quad (\text{S9})$$

We now analyze the asymptotic behavior of  $A_0(r)$  in different regimes.

**Behavior near the Origin ( $r \rightarrow 0$ ):** First, consider the limit  $r \rightarrow 0$ . In this case, both integration bounds converge to the same value:  $(R \mp r)^2 \rightarrow R^2$ . The width of the integration interval vanishes, causing the integral to evaluate to zero.

$$A_0(r) \approx \frac{1}{\pi R^2} \int_{R^2}^{R^2} \dots du = 0. \quad (\text{S10})$$

Thus, the function approaches zero at the origin:

$$\lim_{r \rightarrow 0} A_0(r) = 0. \quad (\text{S11})$$

**Behavior at  $r = R$ :** Next, we evaluate the function at  $r = R$ . The integration bounds become  $(R - R)^2 = 0$  and  $(R + R)^2 = 4R^2$ . Substituting  $r = R$  into the integrand simplifies the expression significantly:

$$A_0(R) = \frac{1}{\pi R^2} \int_0^{4R^2} \sqrt{1 - \frac{(R^2 + u - R^2)^2}{4R^2 u}} du = \frac{1}{\pi R^2} \int_0^{4R^2} \sqrt{1 - \frac{u}{4R^2}} du. \quad (\text{S12})$$

By performing the substitution  $v = u/4R^2$  (which implies  $du = 4R^2 dv$ ), we find:

$$A_0(R) = \frac{4R^2}{\pi R^2} \int_0^1 \sqrt{1-v} dv = \frac{4}{\pi} \left[ -\frac{2}{3}(1-v)^{3/2} \right]_0^1 = \frac{8}{3\pi}. \quad (\text{S13})$$

Thus, the function evaluates to the constant  $8/(3\pi)$  at  $r = R$ .

**Asymptotic Behavior ( $r \rightarrow \infty$ ):** Finally, we examine the limit  $r \gg R$ . We first change the integration variable from  $u$  to  $v = u/r^2$  (so  $du = r^2 dv$ ). The integration bounds  $u = (r \mp R)^2$  become  $v = (1 \mp R/r)^2$ . For  $r \gg R$ , these bounds can be approximated as  $v \approx 1 \mp 2R/r$ . Substituting  $u = r^2 v$  and applying these approximations, the integral becomes:

$$\begin{aligned} A_0(r) &= \frac{1}{\pi R^2} \int_{(1-R/r)^2}^{(1+R/r)^2} \sqrt{1 - \frac{(r^2 + r^2 v - R^2)^2}{4r^2(r^2 v)}} r^2 dv \\ &= \frac{r^2}{\pi R^2} \int_{(1-R/r)^2}^{(1+R/r)^2} \sqrt{1 - \frac{(1 + v - R^2/r^2)^2}{4v}} dv. \end{aligned} \quad (\text{S14})$$

We now expand the integral around  $v = 1$  by setting  $v = 1 + \epsilon$ . For small  $\epsilon$  and  $R/r$ , this expression can be approximated to leading order as:

$$A_0(r) \approx \frac{r}{\pi R} \int_{-2R/r}^{2R/r} \sqrt{1 - \left(\frac{\epsilon r}{2R}\right)^2} d\epsilon. \quad (\text{S15})$$

Defining the new variable  $\beta = \frac{\epsilon r}{2R}$ , which implies  $d\epsilon = (2R/r)d\beta$ , the integral transforms to:

$$A_0(r) \approx \frac{r}{\pi R} \int_{-1}^1 \sqrt{1 - \beta^2} \frac{2R}{r} d\beta = \frac{2}{\pi} \int_{-1}^1 \sqrt{1 - \beta^2} d\beta. \quad (\text{S16})$$

The definite integral  $\int_{-1}^1 \sqrt{1 - \beta^2} d\beta$  evaluates to  $\pi/2$  (the area of a semicircle with radius 1). Therefore, the asymptotic value of  $A_0(r)$  for large  $r$  is:

$$\lim_{r \rightarrow \infty} A_0(r) = \frac{2}{\pi} \left( \frac{\pi}{2} \right) = 1. \quad (\text{S17})$$

### S3. COMPLEX GINZBURG-LANDAU EQUATION

We now derive the continuum equation for the system. The discrete governing equation is given by:

$$\dot{\theta}_i(t) = \omega_i - \frac{K}{4} \sum_{j \in \mathcal{N}(i)} \sin(\theta_i - \theta_j + \alpha). \quad (\text{S18})$$

In the continuum limit, we assume the phase difference between adjacent oscillators is small, i.e.,  $\theta_i - \theta_j \ll 1$ . This permits a Taylor expansion of the sine term:

$$\begin{aligned} \sin(\theta_i - \theta_j + \alpha) &= \sin(\alpha) + \cos(\alpha)(\theta_i - \theta_j) \\ &\quad - \frac{1}{2} \sin(\alpha)(\theta_i - \theta_j)^2 + \mathcal{O}((\theta_i - \theta_j)^3). \end{aligned} \quad (\text{S19})$$

Substituting this expansion into the coupling term of Eq. (S18) yields:

$$\begin{aligned} \frac{K}{4} \sum_{j \in \mathcal{N}(i)} \sin(\theta_i - \theta_j + \alpha) &\approx \frac{K}{4} \left[ 4 \sin \alpha + \cos \alpha \sum_j (\theta_i - \theta_j) \right. \\ &\quad \left. - \frac{1}{2} \sin \alpha \sum_j (\theta_i - \theta_j)^2 \right]. \end{aligned} \quad (\text{S20})$$

To transition to a continuous field  $\theta(\mathbf{r}, t)$ , we approximate the discrete sums using spatial derivatives. First we consider the case of nearest-neighbor coupling ( $R = 1$ ). Assuming a square lattice with spacing  $a$ , the sum of phase differences corresponds to the discrete Laplacian:

$$\sum_{j \in \mathcal{N}(i)} (\theta_j - \theta_i) = \theta_{i+1,j} + \theta_{i-1,j} + \theta_{i,j+1} + \theta_{i,j-1} - 4\theta_{i,j} \approx a^2 \nabla^2 \theta(\mathbf{r}). \quad (\text{S21})$$

where  $a$  denotes the lattice spacing. Therefore,  $\sum_j (\theta_i - \theta_j) \approx -a^2 \nabla^2 \theta(\mathbf{r})$ . Similarly, the sum of squared differences approximates the squared gradient:

$$\sum_j (\theta_i - \theta_j)^2 \approx [(\partial_x \theta)^2 + (\partial_y \theta)^2] = 2a^2 |\nabla \theta|^2. \quad (\text{S22})$$

Substituting these continuous approximations back into the expanded coupling term Eq. (S21) and then into the governing equation Eq. (S18), we obtain the final continuum equation:

$$\partial_t \theta(\mathbf{r}, t) \approx \omega(\mathbf{r}) - K \sin \alpha + D \nabla^2 \theta + \lambda |\nabla \theta|^2. \quad (\text{S23})$$

where  $D = \frac{K}{4} a^2 \cos \alpha$  is the diffusion coefficient and  $\lambda = \frac{K}{4} a^2 \sin \alpha$  is a nonlinear coefficient. This Ginzburg-Landau-type equation reveals the dual role of the phase lag  $\alpha$ , it becomes clear that increasing  $\alpha$  simultaneously reduces the effective diffusion while enhancing the strength of the nonlinear gradient term.

To capture the effects of non-local interactions, we extend the summation to include more neighbors in one dimension. The discrete Laplacian operator is modified by higher-order spatial derivatives. The Taylor expansion of the phase difference  $\theta(x \pm ka)$  up to the fourth order is given by:

$$\theta(x \pm ka) - \theta(x) \approx \pm ka \partial_x \theta + \frac{(ka)^2}{2} \partial_x^2 \theta \pm \frac{(ka)^3}{6} \partial_x^3 \theta + \frac{(ka)^4}{24} \partial_x^4 \theta. \quad (\text{S24})$$

Summing over symmetric neighbors for  $k = 1$  to  $R$  leads to a generalized spatial operator. The expansion yields:

$$\sum_{j \in \mathcal{N}(i)} (\theta_j - \theta_i) \approx \underbrace{\left( \sum_{k=1}^R k^2 \right)}_{D_{\text{geo}}} a^2 \nabla^2 \theta + \underbrace{\left( \sum_{k=1}^R k^4 \right)}_{\gamma_{\text{geo}}} \frac{a^4}{12} \nabla^4 \theta. \quad (\text{S25})$$

For a coupling range of  $R = 6$  and lattice spacing  $a = 0.1$ , the effective geometric coefficients are calculated as  $D_{\text{geo}} = 91a^2 = 0.91$  and  $\gamma_{\text{geo}} \approx 190a^4/12 \approx 0.019$ . Consequently, the inclusion of the fourth-order term  $-\gamma \nabla^4 \theta$  becomes physically essential. This extension yields a Kuramoto-Sivashinsky-type equation governing the phase dynamics.

$$\partial_t \theta \approx \omega - D \nabla^2 \theta - \gamma \nabla^4 \theta + \lambda |\nabla \theta|^2. \quad (\text{S26})$$

#### S4. ENTROPY HYPOTHESIS

To further characterize the system's behavior near the critical point  $\alpha_1$ , we analyze the entropy associated with the topological defects. Unlike the XY model, which is typically described by the Boltzmann entropy  $S = k_B \ln \Omega$ , the topological excitations in our system follow a well-defined probability distribution. Given the previously established relationship for the mean number of defects,  $\bar{n}_+ = ae^{b\alpha}$ , the Shannon entropy is a more appropriate measure.

The Shannon entropy  $S_{\text{Shannon}}$  is thus calculated from the probability distribution  $P(n_+)$  of the number of positive topological defects  $n_+$ :

$$S_{\text{Shannon}} = - \sum_{n_+=1}^{\infty} P(n_+) \ln P(n_+). \quad (\text{S27})$$

To provide a physical basis for the observed defect statistics, we now derive the system's configurational entropy from a micro-statistical perspective. We begin by constructing a microcanonical ensemble to describe the statistical properties of the incoherent core. This system is defined by the incoherent core of radius  $R$  with coherent wave, which we model as a discrete lattice comprising  $N_{\text{core}}$  sites or cells.  $N_{\text{core}}$  is thus proportional to the core's area,  $N_{\text{core}} \propto R^2$ . A macrostate of this system is uniquely defined by the pair  $(N_{\text{core}}, n_+)$ , representing the total number of available sites and the total number of positive topological defects contained within, respectively. The microstates,  $\Omega$ , are the

total number of distinct spatial configurations corresponding to this macrostate. The calculation of  $\Omega$  is a standard combinatorial problem: arranging  $n_+$  indistinguishable topological defects among  $N_{\text{core}}$  distinguishable lattice sites. Assuming a sparse defect population where each site can be occupied by at most one defect, the total number of microstates is given by the binomial coefficient:

$$\Omega_{\text{exact}}(N_{\text{core}}, n_+) = \binom{N_{\text{core}}}{n_+} = \frac{N_{\text{core}}!}{n_+!(N_{\text{core}} - n_+)!} \quad (\text{S28})$$

This exact expression for the microstates is the micro-statistical foundation of the system. The critical insight from this derivation is its direct link to the macroscopic probability distribution  $P(n_+)$ . In the numerical simulations,  $n_+$  is a fluctuating quantity. The incoherent core acts as a system in contact with a "defect reservoir" (the surrounding coherent waves), which is best described by a grand canonical ensemble. In such an ensemble, the probability  $P(n_+)$  of observing  $n_+$  defects depends on both the number of microstates  $\Omega(n_+)$  and the chemical potential  $\mu$  associated with defect creation:

$$P(n_+) \propto \Omega(n_+) e^{\mu n_+} \quad (\text{S29})$$

From this point, the choice of model depends on whether we use the exact  $\Omega$  or an approximation.

**Binomial Distribution:** If we substitute the *exact* number of microstates (Eq. S28) into the grand canonical probability (Eq. S29), we get:

$$P(n_+) \propto \binom{N_{\text{core}}}{n_+} e^{\mu n_+}$$

By defining a parameter  $q = e^\mu$ , the probability is  $P(n_+) \propto \binom{N_{\text{core}}}{n_+} q^{n_+}$ . After normalization, this becomes:

$$P(n_+) = \binom{N_{\text{core}}}{n_+} \left( \frac{q}{1+q} \right)^{n_+} \left( \frac{1}{1+q} \right)^{N_{\text{core}} - n_+}$$

This is precisely the binomial distribution  $B(N_{\text{core}}, p)$ , with the probability of occupation  $p = q/(1+q) = e^\mu/(1+e^\mu)$ . This derivation shows that the binomial distribution is the *fundamental* statistical model for this system, assuming a finite  $N_{\text{core}}$ .

**Poisson Distribution:** Alternatively, if we assume that the defects are sparse, justifying the approximation  $n_+ \ll N_{\text{core}}$ , the expression for  $\Omega$  simplifies significantly. This is the same rare-event condition that underlies the Poisson distribution. Under this approximation, the binomial coefficient becomes:

$$\Omega(N_{\text{core}}, n_+) = \frac{N_{\text{core}}(N_{\text{core}} - 1) \cdots (N_{\text{core}} - n_+ + 1)}{n_+!} \approx \frac{(N_{\text{core}})^{n_+}}{n_+!} = \Omega_{\text{approx}}$$

Substituting this *approximation* for  $\Omega(n_+)$  into Eq. (S29), we find:

$$P(n_+) \propto \frac{(N_{\text{core}})^{n_+}}{n_+!} e^{\mu n_+} = \frac{(N_{\text{core}} e^\mu)^{n_+}}{n_+!}$$

If we define the mean number of defects as  $\bar{N} = N_{\text{core}} e^\mu$ , we recover the functional form of the Poisson distribution:

$$P(n_+) \propto \frac{\bar{N}^{n_+}}{n_+!}$$

This micro-statistical derivation provides a rigorous justification for *both* models. It shows that the binomial distribution is the exact statistical description for a system with a finite number of sites  $N_{\text{core}}$ . The Poisson distribution arises as a valid approximation only under the "sparse defect" condition ( $n_+ \ll N_{\text{core}}$ ), where the finite-size constraint of the core becomes negligible. This explains why our data, which exhibits variance suppression ( $\sigma^2 < \bar{n}_+$ ), is better described by the binomial model. The empirical relation  $\bar{N} = a e^{b\alpha}$  is rooted in the parameter  $\alpha$  controlling both the effective size of the core ( $N_{\text{core}}$ ) and the chemical potential for defect generation ( $\mu$ ).

---

[1] B. Li and N. Uchida, [Phys. Rev. E \*\*104\*\*, 054210 \(2021\)](#).

[2] P.-J. Kim, T.-W. Ko, H. Jeong, and H.-T. Moon, [Phys. Rev. E \*\*70\*\*, 065201 \(2004\)](#).
